# Supplementary material for: Eliminating Order Reduction on Linear, Time-Dependent ODEs with GARK Methods
Source: arXiv:2201.07940 source file (2022-02-14)
Supplement: Supplementary file 1 [file appendix.tex]

%!TEX root=../tc.tex
\subsection{List of Country Apps}
\label{sec:list-country-app}

\begin{table*}[]
\centering
\caption{List of centralized contact tracing approaches and their adoption. *) Contacts are anonymous in France and UK systems; **) Not in France and UK systems; ***) Location can be any source used to locate a user, e.g., GPS coordinates captured by the user's phones or the address of a shop that the user has made a credit card transaction. Personal data can be name, address, gender, or age, etc.
}
\label{tab:ct-centralized}
%\begin{tabular}{|l|l|l|l|l|l|}
\begin{tabular}{llllll}
%\hline
\multicolumn{1}{c}{Approach}                                                                                               & \multicolumn{1}{c}{Tech}                                                                        & \multicolumn{1}{c}{Notification}                                                                       & \multicolumn{1}{c}{\begin{tabular}[c]{@{}c@{}}Data Collected\\ by Server\end{tabular}}                                                                                          & \multicolumn{1}{c}{\begin{tabular}[c]{@{}c@{}}Data Collected\\ by Client\end{tabular}}                                           & \multicolumn{1}{c}{Adoption}                                                                                                                                                                                          \\ \hline
\begin{tabular}[c]{@{}l@{}}BlueTrace \cite{BlueTrace},\\ PEPP-PT \cite{pepppt},\\ TousAntiCovid \cite{TousAntiCovid},\\ CovidRada~\cite{covidradar},\\ E7mi,\\ VirusRadar \cite{virusradar},\\ BlueZone~\cite{BlueZone}\end{tabular} & Bluetooth                                                                                        & \begin{tabular}[c]{@{}l@{}}Server via App/SMS, \\ or the Health Authority \\ via telephone\end{tabular} & \begin{tabular}[c]{@{}l@{}}Users' Temporary \\ identifiers (TempIDs),\\ Who encountered infected users*,\\ Phone number**,\\ Personal data (e.g., \\ name or age)**\end{tabular} & \begin{tabular}[c]{@{}l@{}}TempIDs of the\\ encountered users,\\ Phone number,\\ Personal data (e.g.,\\ name or age)\end{tabular} & \begin{tabular}[c]{@{}l@{}}Australia, France, Singapore, \\ UK (1st version), Czech \\ Republic, Fiji, Gibraltar, \\ Hungary, Malaysia, Mexico, \\ North Macedonia, Philippines, \\ Tunisia, UAE, Vietnam\end{tabular} \\ \hline
\begin{tabular}[c]{@{}l@{}}Rakning C-19~\cite{RakningC19},\\ SafePaths(MIT)~\cite{safepaths-mit}\\ Tawakkalna ~\cite{Tawakkalna},\\ ViruSafe~\cite{ViruSafe},\\ Shlonik~\cite{Shlonik}\end{tabular}                   & Location***                                                                                      & \begin{tabular}[c]{@{}l@{}}Server via App/SMS, \\ or the Health Authority \\ via telephone\end{tabular} & \begin{tabular}[c]{@{}l@{}}Location of all users,\\ Who encountered whom,\\ Phone number,\\ Personal data (e.g., \\ name, age)\end{tabular}                                      & \begin{tabular}[c]{@{}l@{}}Location,\\ Phone number,\\ Personal data (e.g.,\\ name, age)\end{tabular}                             & \begin{tabular}[c]{@{}l@{}}Bulgaria, Cyprus, \\ Kuwait, Saudi Arabia; \\ North Dakota, South \\ Dakota, Wyoming (US)\end{tabular}                                                                                      \\ \hline
\begin{tabular}[c]{@{}l@{}}Aarogya Setu~\cite{AarogyaSetuIndia},\\ BeAware~\cite{BeAwareBahrain},\\ Ehteraz~\cite{Ehteraz},\\ MorChana~\cite{MorChana},\\ PeduliLindungi~\cite{PeduliLindungi} \end{tabular}                    & \begin{tabular}[c]{@{}l@{}}Bluetooth \\ and\\ location\end{tabular}                              & \begin{tabular}[c]{@{}l@{}}Server via App/SMS, \\ or the Health Authority \\ via telephone\end{tabular} & \begin{tabular}[c]{@{}l@{}}Location of all users,\\ Who encountered whom,\\ Phone number,\\ Personal data (e.g., \\ name, age, gender, \\ occupation)\end{tabular}               & \begin{tabular}[c]{@{}l@{}}Location,\\ Phone number,\\ Personal data (e.g.,\\ name, age, gender, \\ occupation\end{tabular}       & \begin{tabular}[c]{@{}l@{}}Bahrain, Bangladesh, India, \\ Indonesia, Qatar, Thailand, \\ Turkey; Rhode Island (US)\end{tabular}                                                                                        \\ \hline
\begin{tabular}[c]{@{}l@{}}Chinese health \\ code system\\ e.g., Hangzhou~\cite{ChinaCTApps}\end{tabular}                                       & \begin{tabular}[c]{@{}l@{}}Combination\\ (Location, \\ credit card \\ transactions)\end{tabular} & \begin{tabular}[c]{@{}l@{}}Server via App/SMS, \\ or the Health Authority \\ via telephone\end{tabular} & \begin{tabular}[c]{@{}l@{}}Location of all users,\\ Who encountered whom\end{tabular}                                                                                            & \begin{tabular}[c]{@{}l@{}}Location,\\ Phone number\end{tabular}                                                                  & China                                                                                                                                                                                                                  \\ \hline
Janus~\cite{istomin2021janus}                                                                                                                        & \begin{tabular}[c]{@{}l@{}}Bluetooth \\ and UWB\end{tabular}                                     & NA                                                                                                      & NA                                                                                                                                                                               & NA                                                                                                                                & NA                                                                                                                                                                                                                     \\ \hline
Hoepman et at.~\cite{hoepman2021hansel}                                                                                                               & Bluetooth                                                                                        & Server via App                                                                                          & TempIDs                                                                                                                                                                          & Encrypted TempIDs                                                                                                                 & NA                                                                                                                                                                                                                     \\ \hline

Buccafurri et at.~\cite{buccafurri2020}                                                                                                                        & \begin{tabular}[c]{@{}l@{}}Location and\\ Bluetooth\end{tabular}                                     & NA                                                                                                      & NA                                                                                                                                                                               & NA                                                                                                                                & NA                                                               \\ \hline                                                                                                                                                

\end{tabular}
\end{table*}

% Please add the following required packages to your document preamble:
% \usepackage{multirow}
\begin{table*}[]
\centering
\caption{List of decentralized contact tracing approaches and adoption.% Exposure status is specified and notified by the App.
}
\label{tab:ct-decentralized}

%\begin{tabular}{|l|l|l|l|l|l|}
\begin{tabular}{llllll}
\hline
\multicolumn{1}{c}{Approach}                                                 & \multicolumn{1}{c}{Tech} & \multicolumn{1}{c}{Notification}                                    & \multicolumn{1}{c}{\begin{tabular}[c]{@{}c@{}}Data Collected\\ by Server\end{tabular}}          & \multicolumn{1}{c}{\begin{tabular}[c]{@{}c@{}}Data Collected\\ by Client\end{tabular}}                       & \multicolumn{1}{c}{Adoption}                                                                                                                                                                                                                                 \\ \hline
\begin{tabular}[c]{@{}l@{}}GAEN~\cite{GAEN:crypto},\\ DP3T-1~\cite{DP3T:WhitePaper}\end{tabular}                         & Bluetooth                 & \begin{tabular}[c]{@{}l@{}}The App notifies \\ the User\end{tabular} & \begin{tabular}[c]{@{}l@{}}Temporary exposure\\ keys (TEKs) of \\ infected users\end{tabular}    & \begin{tabular}[c]{@{}l@{}}TEKs of \\ infected users,\\ TempIDs of the\\ encounter users\end{tabular}         & \begin{tabular}[c]{@{}l@{}}Belgium, Canada, Denmark, \\ Estonia, Finland, Germany, \\ Ireland, Italy, Japan, \\ New Zealand, Northern \\ Ireland, Norway, Poland, \\ Saudi Arabia, South Africa, \\ Switzerland, UK, \\ and 23 states in the USA\end{tabular} \\ \hline
\begin{tabular}[c]{@{}l@{}}DP3T-2~\cite{DP3T:WhitePaper}, \\ MIT-PACT~\cite{PACT-MIT},\\ UW-PACT~\cite{PACT-UW} \end{tabular}                  & Bluetooth                 & \begin{tabular}[c]{@{}l@{}}The App notifies \\ the User\end{tabular} & \begin{tabular}[c]{@{}l@{}}Temporary identifiers\\ (TempIDs) of\\ infected users\end{tabular}    & \begin{tabular}[c]{@{}l@{}}TempIDs of \\ infected users,\\ TempIDs of the \\ encountered users\end{tabular}   & NA                                                                                                                                                                                                                                     \\ \hline
Pronto-B2~\cite{avitabile2020ProntoB2}                                                                      & Bluetooth                 & \begin{tabular}[c]{@{}l@{}} the App notifies \\ the User\end{tabular} & \begin{tabular}[c]{@{}l@{}} Hashed pairs of \\ TempIDs in\\ encounters with \\ infected users\end{tabular}    & \begin{tabular}[c]{@{}l@{}}TempIDs of \\ infected users,\\ TempIDs of the \\ encountered users\end{tabular}   & NA                                                                                                                                                                                                                                                            \\ \hline
\begin{tabular}[c]{@{}l@{}}Co100~\cite{co100},\\ HaMagen~\cite{IsraelHamagen}\end{tabular}                       & Location                  & \begin{tabular}[c]{@{}l@{}}The App notifies \\ the User\end{tabular} & \begin{tabular}[c]{@{}l@{}}Location of \\ infected users\end{tabular}                            & Location                                                                                                      & South Korea, Israel                                                                                                                                                                                                                                           \\ \hline
\begin{tabular}[c]{@{}l@{}}TraceCORONA ~\cite{tracecorona-website},\\ Pronto-C2~\cite{avitabile2020ProntoC2},\\ CleverParrot~\cite{canetti2020cleverParrot}\end{tabular} & Bluetooth                 & \begin{tabular}[c]{@{}l@{}}The App notifies \\ the User\end{tabular} & \begin{tabular}[c]{@{}l@{}}Encrypted encounter \\ tokens (ETs) of \\ infected users\end{tabular} & \begin{tabular}[c]{@{}l@{}}Encrypted ETs of \\ infected users,\\ ETs of the \\ encountered users\end{tabular} & NA                                                                                                                                                                                                                                                            \\ \hline
Epione~\cite{trieu2020epione}, \\ Dittmer et al. \cite{dittmer2020}                                                                         & Bluetooth                 & \begin{tabular}[c]{@{}l@{}}The App notifies \\ the User\end{tabular} & TempIDs of infected users                                                                        & \begin{tabular}[c]{@{}l@{}}TempIDs of the\\ encountered users\end{tabular}                                    & NA                                                                                                                                                                                                                                                            \\ \hline
\end{tabular}
\end{table*}

\noindent\textbf{List of centralized approaches.}
\label{sec:list-centralized-app}
Table~\ref{tab:ct-centralized} shows an overview of prominent centralized contact tracing solutions. \changeT{In the table, the apps are categorized by employed technology, e.g., notification method and type of data collected. Further, adoption information is also provided, from which one can see that centralized-based approaches are more preferred in Asian countries than on other continents. In terms of technologies, besides Bluetooth, location is also widely used in many countries. Noticeably, many if not most deployed apps, e.g., \cite{BlueTrace, covidradar, AarogyaSetuIndia}  collect sensitive data, e.g., phone numbers, names, ages of the users.}  

It is worth noting that some schemes have been proposed to improve the security and privacy of centralized approaches \cite{hoepman2021hansel, istomin2021janus}. For example, Hoepman et al. \cite{hoepman2021hansel} propose two centralized protocols that aim to reduce the risk of tracking users’ locations and replay attacks. The first handshake (peer-to-peer) protocol establishes logs of encounters. In particular,  $\useri$ broadcasts a public key, and $\userj$ in the vicinity will respond with $\userj$’s ID encrypted by $\useri$’s public key and vice-versa.  However, this peer-to-peer protocol fails if either of the two-way messages is lost. Therefore, Hoepman et al. introduce a second approach that utilizes a central server to tackle this issue so that devices only need to broadcast a random public key. The responses with encrypted ID information will then be sent via the server, i.e., do not need to be sent directly via the BLE channel.

%%%%%%%%%%%%%%%%%%%%%%%%%%%%%%%%%
\noindent\textbf{List of decentralized approaches.}
\label{sec:list-decentralized-app}
Table~\ref{tab:ct-decentralized} shows an overview of prominent solutions. \changeT{It shows that most approaches use Bluetooth, some use location while a very few approaches using other technologies, e.g., \cite{istomin2021janus} using UWB and \cite{MIT-SonicPACT} using ultrasound.  
Further, the figure shows that \gap is widely used in Western Europe and North America while South Korea and Israel use their own location-based approaches. Unfortunately, other decentralized approaches that claim to have better security and privacy guarantees in comparison to \gap, e.g., Pronto-C2\cite{avitabile2020ProntoC2}, ClerverParrot\cite{canetti2020cleverParrot}, and Epione \cite{trieu2020epione} have not been adopted yet. In terms of data collection, decentralized apps do not collect personal data of users like phone numbers, email addresses or names. However,  the system (consisting of $\service$ and Apps) collects encounter information of infected users and additionally, the apps also record information about encounters with other users in the vicinity. Such encounter information can be generally divided into two categories based on which cryptographic approach is used. Apps based on the use of symmetric cryptography collect temporary IDs ($\tempId$s) of other users and match these against IDs that they derive from the temporary exposure keys ($\tek$s) of all infected users they download from $\service$. In contrast, apps based on asymmetric cryptography establish encounter-specific cryptographic tokens for each encounter. To enable identification of at-risk encounters, infected users upload hashed values of their encounter tokens to $\service$, from where all other users download them and compare them to the hashed versions of their collected encounter tokens. In case there is a match, this is an indication that an at-risk encounter with an infected person has taken place.}

\subsection{Advanced Privacy Techniques}
\label{sec:privacy-tech}

There are several (mainly cryptography-based) privacy techniques that have been considered to enhance privacy of \dct. Table \ref{tab:advanced-pri-tech} shows an overview of such approaches. Unfortunately, none of these contact tracing approaches have been used in practice yet. Next, we will elaborate on these approaches. 

\noindent\textbf{Blind Signature.} Some approaches, e.g., \cite{reichert2021ovid, avitabile2020ProntoC2} propose using a blind signature scheme to verify the authenticity of encounter information, e.g., the temporary keys that infected users upload to the tracing service provider $\service$. In contrast to common approaches in which $\healthauthority$ gives a unique transaction number (TAN) to each of the infected users for uploading their data, allowing $\healthauthority$ to link infected users in a \dct to $\healthauthority$'s patient data, blind signature-based approaches prevent this by enabling $\healthauthority$ to "blindly" sign the temporary keys of infected users without knowing the actual content. Therefore, neither $\healthauthority$ nor any other party can know based on verification information to which user of the system published temporary keys belong.

\noindent\textbf{Blockchain.} Instead of using a centralized server to collect and forward encounter information of infected users to other users, some approaches by, e.g., Avitabile et al. \cite{avitabile2020ProntoC2} or Hasan et al. \cite{ Hasan2021blockchain} leverage a blockchain to decentralize the process of publishing, verifying, and matching encounter information. This makes the system transparent to users in that it does not require a trusted server.

\noindent\textbf{Private Set Intersection (PSI) and binary filters.} The core function of a \dct app is to find a match between encounter information of infected users and other users. However, this process raises privacy concerns.
In centralized approaches, $\service$ has access to encounter information of all infected users, whereas in decentralized approaches, any user can receive information about the encounters of all infected users, providing the potential for possibly inferring information about the user's location and social graph. To solve this problem, Trieu et al.~\cite{trieu2020epione} and Dittmer et al.~\cite{dittmer2020} leverage a private set intersection (PSI) approach utilizing Function Secret Sharing (FSS) techniques \cite{boyle2015function}.
The idea is that $\service$ (which has a set of $\tempId$s of all infected users) and a potentially affected user $\userj$ (who has a set of $\tempId$s of the users whom $\userj$ has encountered) collaborate to perform encounter matching in a way that only the matching results (e.g., the number of matching $\tempId$s) become known to $\userj$. 
This means that $\service$ does not get to know encounter information of $\userj$ (e.g., $\tempId$s) and vice versa.
However, a PSI-based approach often incurs high computation and communication overhead which makes it less practical. A more simple approach is to use a  cuckoo filter~\cite{DP3T:WhitePaper}, where the $\service$ builds a filter from the $\tempId$s of the infected users and sends it to user Apps. Apps can check for matches by inputting each of their observed $\tempId$s into the filter and receive an output whether the $\tempId$ is in the filter or not. Thus, Apps can do matching without having access to the complete list of $\tempId$s of infected users.

\noindent\textbf{Secret Sharing.} In order to prevent $\tempId$s to be captured or relayed easily, Troncoso et al.~\cite{DP3T:WhitePaper} propose to use secret sharing by dividing a $\tempId$ into $n$ parts, so-called secret shares that are broadcast into the user's vicinity over time. This means that any other user needs to remain in vicinity of the user to capture at least $k$ out of $n$ shares to be able to reconstruct the $\tempId$, making it more difficult for an adversary to stage successful attacks by just relaying $\tempId$s of people passing by them. \fixedMC{However, this approach has several limitations and drawbacks. Firstly, this approach is ineffective in main attack scenarios like shopping, public events or restaurants where adversary has enough time to capture at least $k$ shares. Secondly, this approach would introduce a significant overhead, latency, and error rate because it requires from $k$ to $n$ times more communication overhead (compared to BlueTrace or \gap) and significant computation to reconstruct the $\tempId$ from the shares. Further, the authors argue that the communication overhead is insignificant if the number of shares is equal to the number of broadcasts that the App makes within an epoch (the lifetime of a $\tempId$). However, this is a flaw as many encounters would not be recorded if the encounters do start at the beginning of the epoch.}

\noindent\textbf{Use of Anonymization Networks.} A malicious $\service$ may track IP addresses of users uploading and downloading encounter information, which potentially could (1) leak personal information of the user, e.g., home addresses and (2) be used to link users with encounter information they upload. Therefore, a number of existing approaches (e.g., \cite{castelluccia2020desire}) propose to use an anonymization network like Tor or a Mixnet to prevent such potential leakage.

\begin{table}[]
    \centering
    \caption{Advanced privacy techniques for DCT systems}
    \begin{tabular}{l|l}
    Techniques & References \\ \hline
    Blind signature & \cite{reichert2021ovid, avitabile2020ProntoC2} \\
    Blockchain & \cite{avitabile2020ProntoC2, Hasan2021blockchain} \\
    Private set intersection/ a filter         &  \cite{trieu2020epione, dittmer2020, berke2020assessing, OpenMined2020maximizing, DP3T:WhitePaper}\\
    Secret sharing &  \cite{DP3T:WhitePaper} \\ 
    Tor/Mixnet & \cite{castelluccia2020desire} \\
    Others & \cite{cheng2020KHOVID}\\ \hline
    \end{tabular}
    
    \label{tab:advanced-pri-tech}
\end{table}

\subsection{Other Application Scenarios of \ourname}
\label{sec:discussion}
%!TEX root=../tc.tex

\noindent\textbf{Smartphone and Wearable Devices.}
\label{sec:wearable}
Smartphones are prohibited or inconvenient to use in many scenarios like in schools, hospitals, corporate offices, sports and other events, beaches, waterparks, funfairs, etc. Therefore, we propose using wearable devices as a complementary approach for contact tracing. Figure \ref{fig:wristband} shows our smartband-based \ourname. The Bluetooth tracing function is integrated in the smartbands to emit and record the Ephemeral Public Keys $Q$s and ephemeral IDs which are generated by the \app{s} on the smartphones. The smartphones are also responsible for calculating ETs $k$s from private key $d$s and public key $Q$s collected by the smartbands. The protocol is summarized as follows:

\begin{enumerate}
	\item The smartphones generate ECDH private key $d$s and public $Q$s, and ephemeral IDs $EI$s for the next day or the next few days.
	\item The smartphones send $Q$s and $EI$s to the smartbands every day or every few days or when users interact with the apps. 
	\item The smartbands exchangse $Q$s and $EI$s with other devices (smartbands or smartphone tracing apps) in vicinity.
	\item The smartbands send $Q'$s and $EI'$s that they have received from other devices along with associated metadata (timestamp and duration) to the smartphones.
	\item The smartphones calculate the ETs from their own private keys $d$s and other public keys $Q'$s.
	\item The smartphones perform all other phases: infection verification, token information upload and token information download.	
\end{enumerate}  

In order to avoid double encounter recording as both the phone and its pair smartband exchange public keys to other devices in vicinity, the system can detect the co-presence of two devices using a separate secure Bluetooth channel (since both the phone and the smartband are paired) and let only one of the devices perform tracing. In case the phone and its pair smartband are our of range, the smartband will run the tracing functionality but the phone can pop-up a message to ask user whether they prefer do tracing on the phone or not, e.g., if the smartband is running out of battery.

\begin{figure}
	\centering
	\includegraphics[width=\columnwidth]{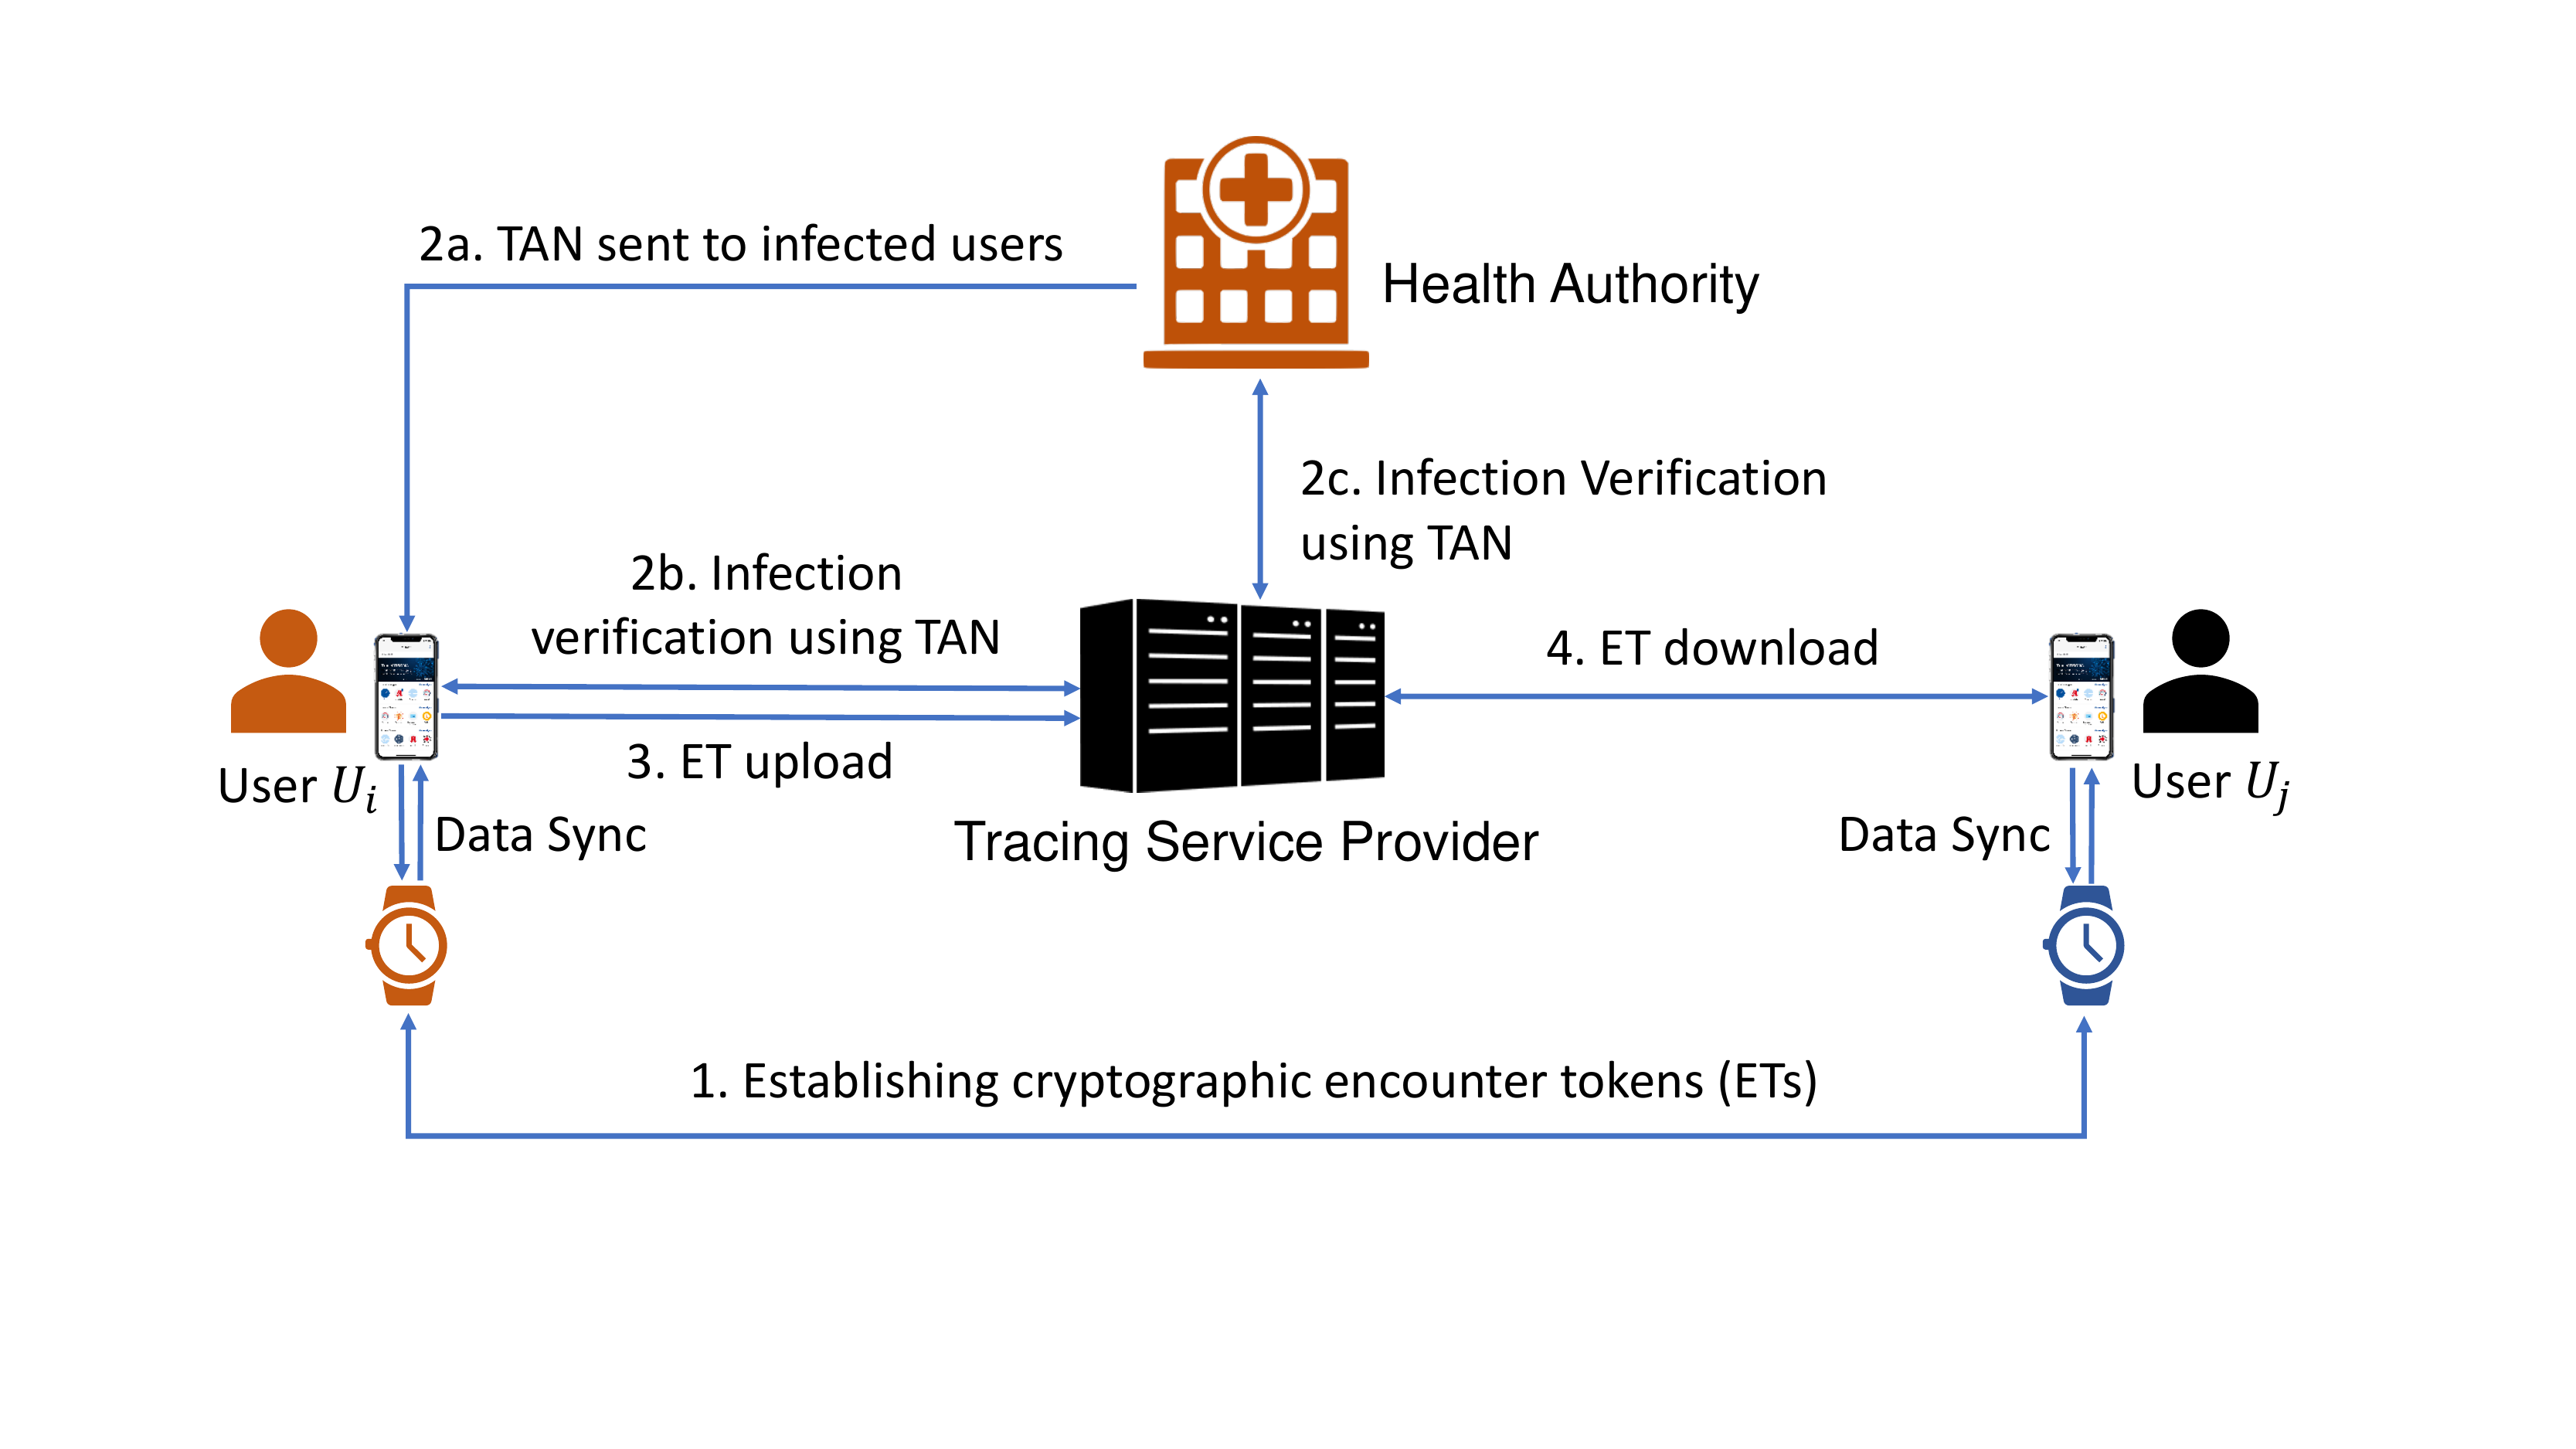}
	\caption{TraceCORONA system using wristband.}
	\label{fig:wristband}
\end{figure}

The wearable device and the smartphone frequently synchronize their data, so that the smartphone sends the $Q$s that it generates to the wearable device and the wearable device sends the $Q'$s it has received from other devices in proximity along with metadata associated with them to the smartphone. This synchronization function can be executed periodically, e.g., daily or when the phone is being charged or when the user interacts with the \ourname app, i.e., when the app is running in the foreground. For one day, the smartphone sends 96 $EI$s and 96 $EPK$s ( 24 hours x 4 EPKs/hour if $T = 15$ minutes). In total, the phone sends 96x(65+520) = 56,064 (bits) or 58 kbits. The amount of data that the wearable device sends to the phone depends on how much encounters (contacts) a user has during the day. Recent research shows that on average, a user has about 20 contacts (with a duration over 15 minutes) with other users excluding household members. Therefore, we estimate that the wearable device sends ca. 31 kbits to the phone daily. In theory, Bluetooth LE can transfer from 125 kbit/s to 2 Mbit/s meaning that the daily synchronization process can be done in seconds.

\noindent\textbf{Proximity Communication.} In this paper, we focus on Bluetooth Low Energy (Bluetooth LE) as a prominent example. However, \ourname can work with any type of short-range wireless communication protocols like ZigBee or Z-Wave. Further, other communication protocols or data transfer channels like NFC (Near Field Communication), ultrasound or QR code can also be used.  
   
\noindent\textbf{Public and Private Contact Tracing Systems.}
Many organizations like schools or corporations have needs for performing contact tracing that do not necessarily align well with the needs and requirements of a national or country-level tracing solution \cite{Salesforce2020Private, IBM2020Private}. Many businesses and organizations would like to implement their own (private) tracing solutions to have the flexibility of better managing quarantining of employees. To tackle this problem, some manual private contact tracing solutions, e.g., \cite{Salesforce2020Private} have been introduced. \ourname is flexible in the sense that it can be applied to private contact tracing directly. For example, a \ourname service provider can provide infrastructure (e.g., the server, the apps and dashboard control) to organizations or corporations for a private deployment. Since administrators like personnel departments know who in their organizations or companies are tested positive for COVID-19, they can issue $TAN$s and verify infection state as explained in Sect. \ref{sec:verification-upload}. Further, our smartband tracing solution can also help to cover many use cases in which using smartphones is forbidden e.g., in many schools or companies as mentioned above.

%%%%%%%%%%%%%%%%%%%%%%%%
% put here so that it will be shown in the next page.
%We summarize attacks on \dct in Tab. \ref{tab:existing-attacks-analyses}.
\begin{table*}[]
\centering
\caption{Attacks and analyses on existing contact tracing approaches. IDU: Identifying Users, PIU: Profiling Infected Users, ISC: Inferring Social Graph, FEC: Fake exposure Claim, RA: Relay Attack, DCT: Digital Contact Tracing.}
\label{tab:existing-attacks-analyses}

\begin{tabular}{|l|c|c|c|c|c|c|l|l|}
\hline
\multicolumn{1}{|c|}{}                         & IDU & PIU & ISC & FEC & RA & Effectiveness & \multicolumn{1}{c|}{Other}                                    & \multicolumn{1}{c|}{Target}                                              \\ \hline
Avitabile et al., \cite{avitabile2020ProntoC2}   & x   & x   & x   &     & X  &               &                                                               & \begin{tabular}[c]{@{}l@{}}GAEN\\ DP3T-1\\ PEPP-PT\\ ROBERT\end{tabular} \\ \hline
Avitabile et al., \cite{avitabile2020tenku}    &     &     &     &     & X  &               &                                                               & GAEN                                                                     \\ \hline
Baumgaertne et al., \cite{baumgartner2020mind} &     & x   & x   &     & x  &               &                                                               & GAEN                                                                     \\ \hline
Boutet et al., \cite{ourPamphlet}              & x   & x   & x   & x   & x  &               &                                                               & GAEN                                                                     \\ \hline
Crocker et al., \cite{crocker2020challenge}    & x   & x   & x   &     & x  & x             &                                                               & GAEN                                                                     \\ \hline
Danz et al., \cite{danz2020security}           & x   & x   & x   &     & x  &               &                                                               & \begin{tabular}[c]{@{}l@{}}GAEN\\ DP3T-1\end{tabular}                    \\ \hline
Dehaye et al., \cite{dehaye2020swisscovid}     &     &     &     &     & x  &               &                                                               & GAEN                                                                     \\ \hline
Gennaro et at., \cite{Gennaro2020}             &     &     &     &     & x  &               &                                                               & GAEN                                                                     \\ \hline
Gvili et al., \cite{gvili2020security}         & x   & x   & x   & x   & x  &               & DoS*                                                          & GAEN                                                                     \\ \hline
Iovino et al., \cite{Iovino2020timetravel}     &     &     &     &     & x  &               &                                                               & GAEN                                                                     \\ \hline
Kojaku et al., \cite{kojaku2020effectiveness}  &     &     &     &     &    & x             &                                                               & GAEN                                                                     \\ \hline
Lanzing et al., \cite{lanzing2020ethical}      &     & x   & x   &     &    &               & \begin{tabular}[c]{@{}l@{}}Monopolist\\ Coercion\end{tabular} & GAEN                                                                     \\ \hline
Leith et al., \cite{leith2020coronavirus}      &     &     &     &     &    & x             &                                                               & Bluetooth                                                                \\ \hline
Leith et al., \cite{leith2020gaendata}         & x   & x   & x   &     &    &               & Data collection                                               & GAEN                                                                     \\ \hline
Vaudenay et al., \cite{vaudenay2020analysis}   &     & x   &     &     & x  &               &                                                               & \begin{tabular}[c]{@{}l@{}}GAEN\\ DP3T\end{tabular}                      \\ \hline
Vaudenay et al., \cite{vaudenay2020dilemma}    & x   & x   & x   & x   & x  &               &                                                               & \begin{tabular}[c]{@{}l@{}}GAEN\\ DP3T\\ PEPP-PT\end{tabular}            \\ \hline
Wen et al., \cite{Wen2020study}                &     &     &     &     &    & x             & Data collection                                               & 41 apps                                                                  \\ \hline
White et al., \cite{White2021why}              & x   & x   & x   &     &    & x             & \multicolumn{1}{c|}{}                                         & DCT                                                                      \\ \hline

White et al., \cite{white2021privacy}                & x     & x     &  x   &     &    & x             & Ethics                                               &  \dct                                                                 \\ \hline
\end{tabular}
\end{table*}

%%%%%%%%%%%%%%%%%%%%%%%%%%
\subsection{Parameter Settings and Estimations}
\label{sec:parameters}
We now analyze the data use of the \ourname protocols and define following parameters for our analysis.
\begin{itemize}
	\item $EI$ - Ephemeral Identification (128 bits). $EI$ is used to temporarily identify devices in proximity.
	item $Q$ - Ephemeral ECDH Public Key (384 bits). $Q$ is used together with associated secret keys to establish encounter tokens. 
	\item $UUID$ - Universally Unique Identifier (128 bits). $UUID$ is used to identify the \ourname app.
	\item $ET$ - Encounter Token (256 bits). $ET$ is used to uniquely identify the encounter between two users.		
	\item $AM$ - Advertising Message (256 bits). $AM$ is used to advertise (broadcast) $UUID$s and $EI$s of devices. It changes every $T$ minutes.
	\item $RSSI$ - Received Signal Strength Indicator.	$RSSI$ indicates the strength of a received Bluetooth signal that can be roughly used to estimate the distances between the sender and the receiver.
\end{itemize}

In the following, we present estimation of data exchange (network bandwidth) and key parameters. %\todo[inline]{Which section? The follow up section Proximity Identification? Not understandable}

\noindent\textbf{Proximity Detection.} Each \ourname App constantly advertises and scans for $AM$ messages. We aim to make sure that a device records other devices in proximity every 2 minutes. The app periodically advertises $AM$s  every minute, during which devices run Bluetooth LE advertising for 40 seconds and are in idle mode for 20 seconds. The app periodically scans $AM$s every 50 seconds, during which devices run Bluetooth LE scanning for 30 seconds and are in idle mode for 20 seconds. These advertising and scanning patterns are empirically selected to ensure that \ourname keeps track of other devices every 2 minutes.   

\noindent\textbf{Public Key Exchange.} When a device finds a new device in proximity, the two devices start exchanging public key $Q$. First, one device starts the Bluetooth client and another device starts the Bluetooth server and both devices exchange their public keys $Q$s (384-bit length). Both devices store the $Q$s which later on are used to calculate $ET$s. $Q$ is changed every $T$ minutes along with $EI$. During a $T$-minute lifetime, to save energy, $Q$ is only sent when the device finds a new device.

\noindent\textbf{Encounter distance - 2 meters.}
In theory, the Bluetooth Low Energy (BLE) signal range is up to 50 meters. In the context of contact tracing, we consider the distance of two meters or smaller.

\noindent\textbf{Encounter time – 15 minutes.}
The encounter time that is equal to or more than 15 minutes should be considered as a high exposure risk. 

\noindent\textbf{Expected number of Encounter Tokens per day - 20.}
In average, a user has approximately 16 encounters (15 minutes or longer) with other users excluding known contacts e.g., household members or colleagues in the same office \cite{DelValle2007}. %\todo[inline]{Is this parameter reasonable? Any studies on this? Added a reference.}

\noindent\textbf{Amount of data uploaded by the app to the server – 4.3 kB.}
The app of the infected user uploads the hashes (128 bits) of $ET$s for 14 days (20 $ET$s per day as mentioned above). Hence, the total amount of data should be, 14*20*128 = 35,840 (bits) or 4.3 (kB).

\noindent\textbf{Amount of data downloaded by the app from the server – 8.6 MB per day.}
If we assume there are 10,000 new COVID-19 cases per day, the app will download 10,000* 4.3 = 43,000 (kB) or 43 MB per day.

\noindent\textbf{Amount of data received by the server (daily) – 43 MB per day.}
The same to the data that an app downloaded.

\noindent\textbf{Amount of data sent by the server (daily) – 2150 TB per day.}
If we assume that there are 50 million app users, the server will send 50,000,000* 43 = 2,150,000,000 (MB) or 2150 TB per day.

\noindent\textbf{Maximum numbers of devices in proximity that the App can establish the Encounter Tokens per second - 100.}
In theory, we can estimate the amount of encounter established based on the bandwidth of BLE communication. To establish an $ET$, the device need to send and receive an AM and $Q$ that are 192 + 520 = 712 (bits) or 712 *2 = 1,424 (bits) for both sending and receiving. In the worst case, the BLE bandwidth is 125 (kbit/s) that means the app can establish 125,000/ 1,424 = 175 $ET$s per second. In the ideal case, the BLE bandwidth is 2 Mbit/s that means the app can establish 2,000,000/1,424  = 1,404 $ET$s per second. However, since the latency to establish a BLE connection is ca. 6 ms, the app can only establish 1000/6 = 160 $ET$s per second if we consider the data transmission time is much smaller than the connection time. Thus, it is fair to estimate that the app can establish 100 encounters per second.

\subsection{List of Existing Works on  Digital Contact Tracing}
\label{sec:existing-analysis}
We summarize attacks on \dct in Tab. \ref{tab:existing-attacks-analyses}.
